# Supplementary material for: When Can Transformers Ground and Compose: Insights from Compositional Generalization Benchmarks
Source: arXiv:2210.12786 source file (2022-10-31)
Supplement: Supplementary file 1 [file architecture.tex]

\begin{figure*}[t]
	\centering
	\includegraphics[scale=1.2]{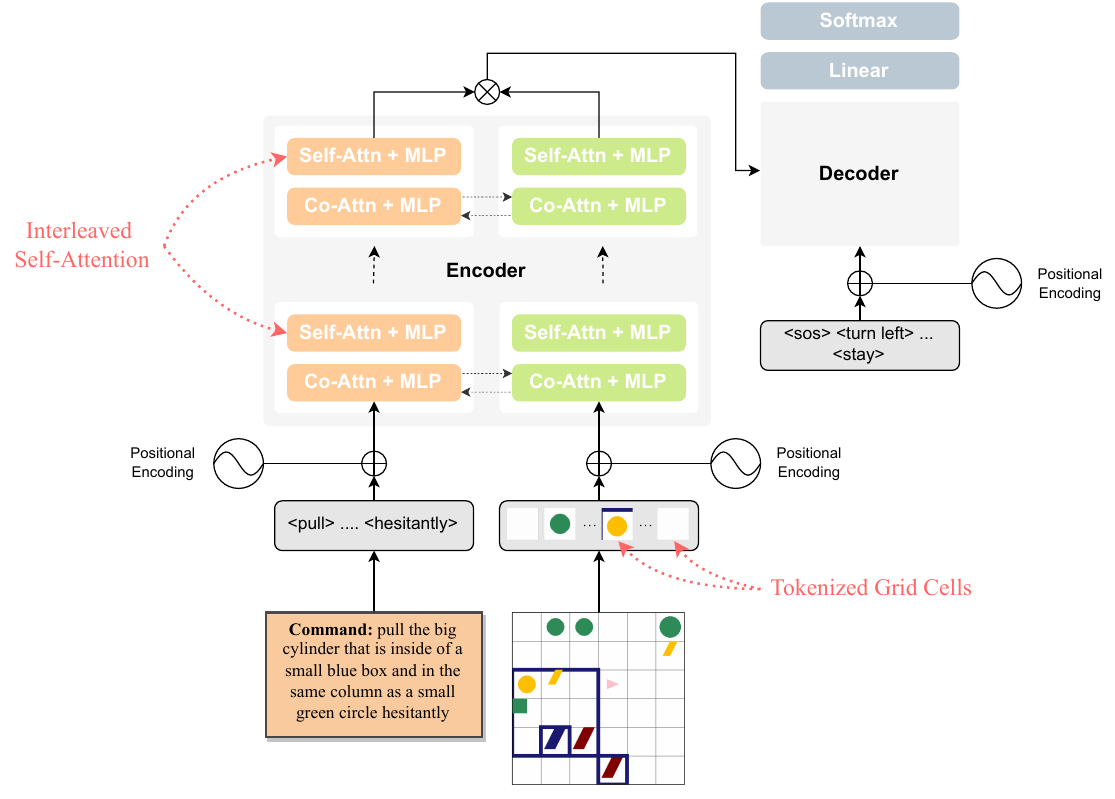}
	\caption{\label{fig:moddel} An example from the \texttt{direct-grounded} experiment on LLMs.}
\end{figure*}
